# Supplementary material for: Broadband and wide-angle beam deflection enabled by dynamically reconfigurable meta-arrays
Source: arXiv:2510.17075 source file (2025-10-20)
Supplement: Supplementary file 1 [file supplemental_information_updated.pdf]

# Broadband and wide-angle beam deflection enabled by dynamically reconfigurable meta-arrays

**KOFFI-EMMANUEL SADZI AND ABDOULAYE NDAO***

University of California, San Diego, Department of Electrical and Computer Engineering, La Jolla, California, United States

*a1ndao@ucsd.edu

## SUPPLEMENTAL MATERIAL

### Section A. Optical property of the Antimony Trisulfide (Sb2S3)

The performance of the dynamically tunable broadband deflector depends on the optical properties of the crystalline and amorphous phases of the antimony trisulfide, Sb2S3. Using ellipsometry, we measured the (n, k) data of Sb2S3 for a wavelength range of 300 nm to 2500 nm for both crystalline and amorphous states. The results are presented in **Fig.S1**.

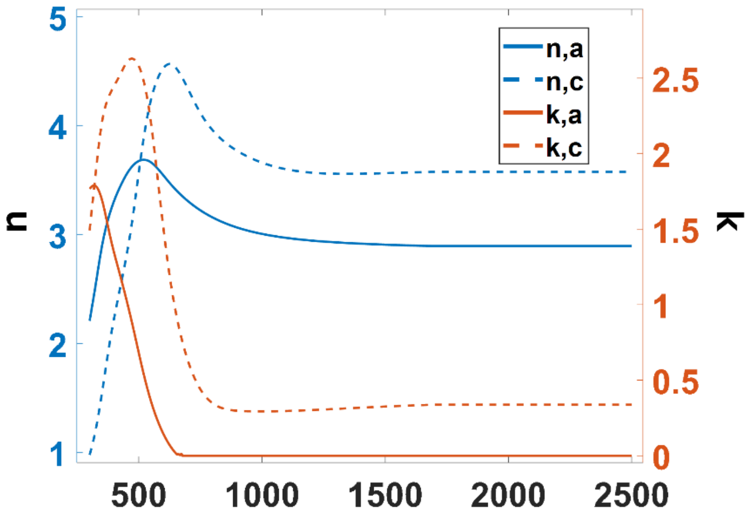


*Figure S1 Real (n) and imaginary (k) part of the refractive index for the crystalline (shorted to "c") and amorphous (shorted to "a") phase of SbS3*

## Section B. Effect of Capping layer on the performance of the device

To prevent oxidation of sulfur in $Sb_2S_3$, the device is capped with a $SiO_2$ layer of thickness t, which we investigate over the range of 15–45 nm, consistent with typical values reported in the literature [1,3–6]. Figure S2 shows the unit cell of the $SiO_2$-capped device. Simulations across both crystalline and amorphous states, and for incidence angles of 30°, 45°, and 60°, reveal that the capping layer has minimal impact on performance. In the crystalline state, the first-order deflection coefficient varies by less than 1% on average (Fig.3b), and the passband reduction is at most 2.1% (Fig.3a). In the amorphous state, deflection variations remain around 2% on average (Fig.4b), and the passband reduction stays below 2% (Fig.4a). These results demonstrate that the device maintains exceptional stability and robustness across a wide range of capping thicknesses.

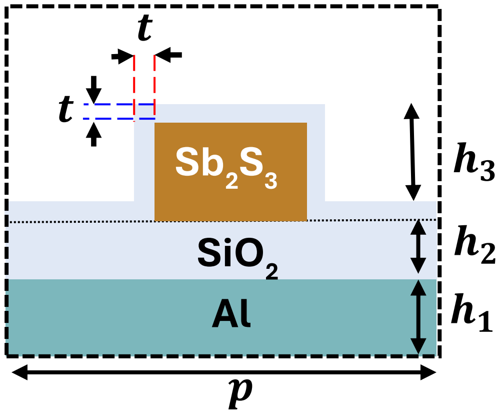


Figure S2 Unit-cell of the broadband deflector with SiO2 capping layer

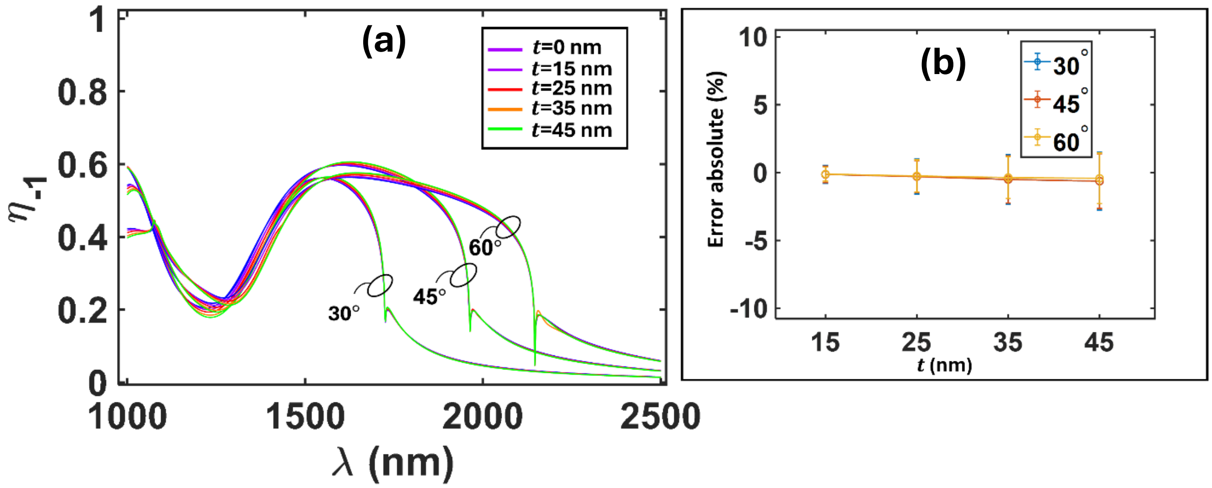


*Figure S3 (a) effect of the capping layer on the performance of the broadband wide-angle deflector, in the crystalline state. (a) Statistics of the deviation in $\eta_{-1}$ for capping layer of thickness t with respect to the un-capped device.*

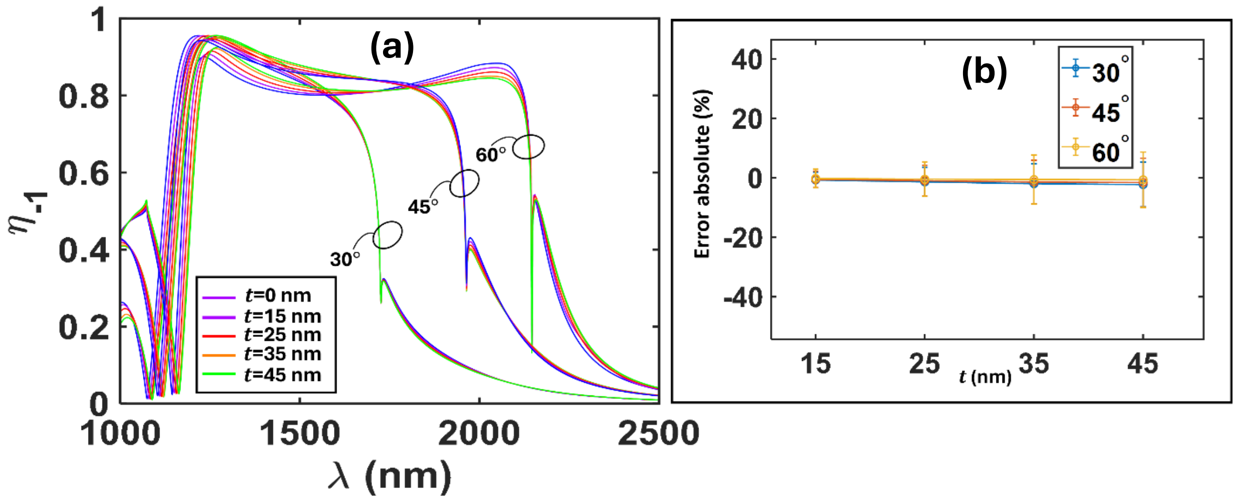


*Figure S4 (a) effect of the capping layer on the performance of the broadband wide-angle deflector, in the amorphous state. (b) Statistics of the deviation in $\eta_{-1}$ for capping layer of thickness t with respect to the un-capped device.*

## Section C. Results of parameter sweep for optimal device

*Simulation setup:*

Simulations were performed using SIMULIA Computer Simulation Technology (CST) with a three-dimensional full-wave solver based on the finite element method (FEM). The system was modeled as a unit cell in the XY plane with Floquet boundary conditions and a frequency-domain solver. On one hand, the lower boundary ($z_{\min}$) was initially set to open and later replaced by a PEC after confirming that the chosen aluminum layer thickness fully blocked transmission, enabling faster computation. The upper boundary ($z_{\max}$) was kept open, with the distance to the reference planes set to $\lambda_{\text{mid}}/2$, where $\lambda_{\text{mid}}$ = 1700 nm corresponds to the central wavelength of the 1000–2500 nm operating range. TE or TM polarizations were applied as appropriate, and the first seven Floquet modes were considered to analyze diffraction. Incidence angles were controlled via the scan-angle parameter. Convergence was ensured by imposing a relative residual below $10^{-4}$ for all Floquet modes and an all-S-parameter interpolation error under 0.1.

*Sweep results and Analysis considerations:*

The following targets led the parameter search for the design of the deflector: a large difference between the coefficient of deflection of the -1st order in the crystalline and amorphous cases, a wide passband, and wide-angle coverage. Further consideration is to ensure a sharp change at the cutoff wavelength of the broadband deflector, which is of interest for spatial filtering.

In the analysis of the spectrum of the deflection coefficient $\eta_{-1}$, Fig. S5 (a) and (b) show that the upper bound of the passband increases with the period p, for crystalline and amorphous states of the **$Sb_2S_3$** strip, respectively. This supports Eq. (1), which is also presented in the main manuscript, which describes the angle of reflection of different diffraction orders. From Eq. (1), the reflected wave of order n propagates when $|sin\ (\phi_n\ )| \leq 1$. Therefore, for an increasing period $p$, more wavelengths ($\lambda$) are supported, particularly for n=-1. Eq. 1 also implies that the diffraction limit increases with the incidence angle θ. Based on Fig. S7, $p$ = 1150 nm was chosen as a mid-value

between 1100 nm and 1200 nm, as it balances a sharp cutoff and a flat passband, with more relevance given to the amorphous state-based simulation.

$$\sin \phi_n = \sin \theta + n \frac{\lambda}{p} \qquad (1)$$

Moreover, Fig. S6 (a) and (b) show that the lower bound of the passband increases with the height of the Sb2S3 $h_3$, for crystalline and amorphous states of the Sb2S3 strip, respectively. This reduces the passband of the device, making it more selective. To ensure a lower bound with a sharp edge at the start of the O-band (1260 nm-1360), $h_3 = 200$ nm is chosen.

Finally, the thickness $h_2$ of the $SiO_2$ plays a crucial role in the power attenuation functionality of the device as it controls the maximum value of $\eta_{-1}$ . Figure S7 (a) and (b) show its effect on the spectrum of the deflection efficiency. In the crystalline case (Fig. S7 (a)), efficiency drops with increasing $h_2$ .In contrast, for the amorphous case (Fig. S7 (b)), the flatness or the uniformity of the deflected power is altered with the decreasing value of $h_2$. Hence, although we would like a very low deflection coefficient $\eta_{-1}$ under the crystalline condition, $h_2$ = 60 nm represents a compromise choice to tolerate a maximum drop of 20% in the passband regime across the different incident angles. Importantly, all the final parameters are chosen to allow also a margin for fabrication error.

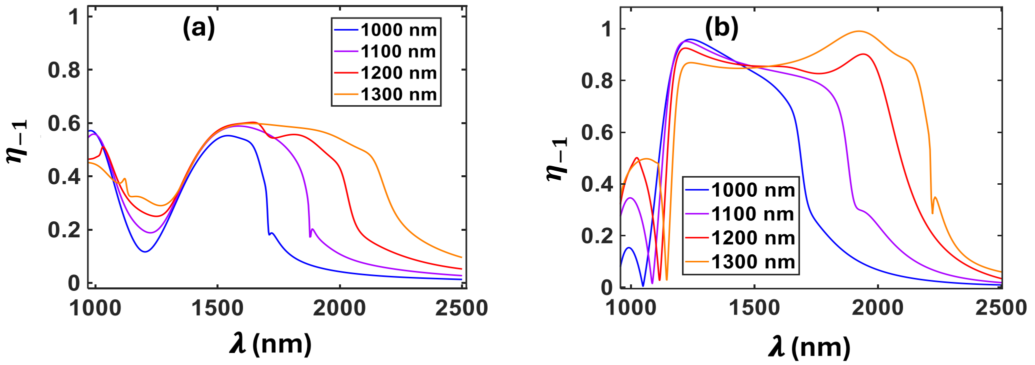


*Figure S5. Effect of the period p of the structure on the spectrum of the -1st order deflection, for the PCM in crystalline (a) and amorphous (b) states; $\theta_{inc}$ =45°.*

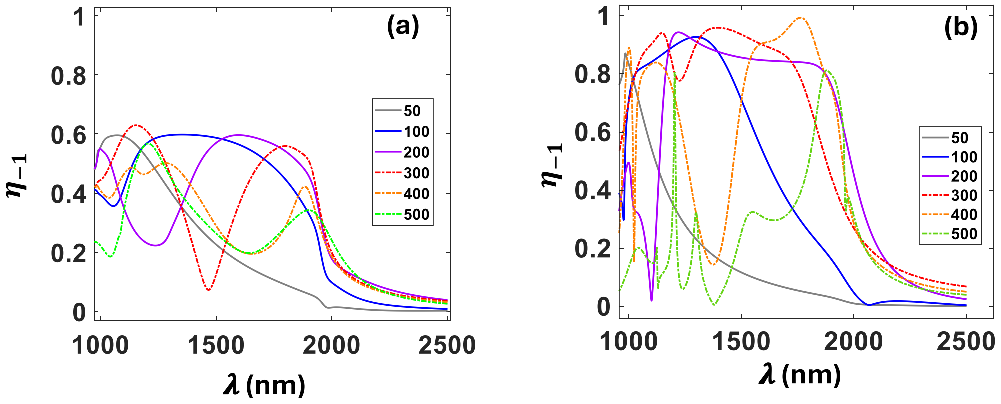


*Figure S6. Effect of the height of the Sb2S3 $h_3$ on the spectrum of the -1st order deflection, for the PCM in crystalline (a) and amorphous (b) states; $\theta_{inc}$=45°.*

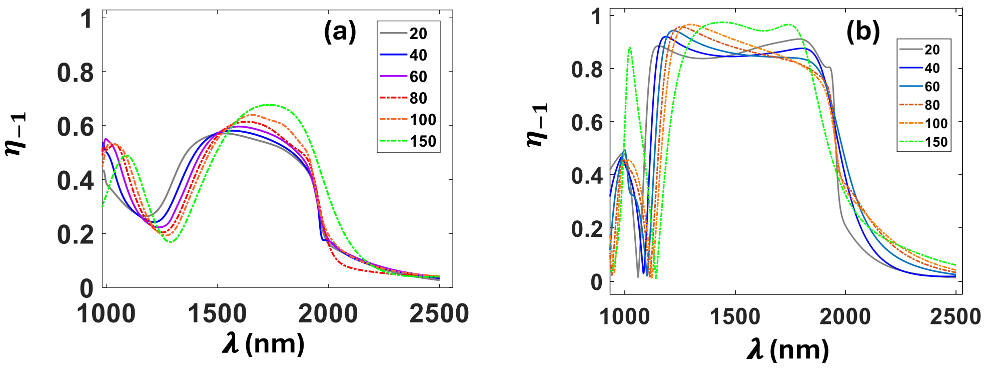


*Figure S7. Effect of the height of the SiO2 $h_2$ on the spectrum of the -1st order deflection, for the PCM in crystalline (a) and amorphous (b) states; $\theta_{inc}$=45°.*

## Section D. Fabrication process of the broadband deflector

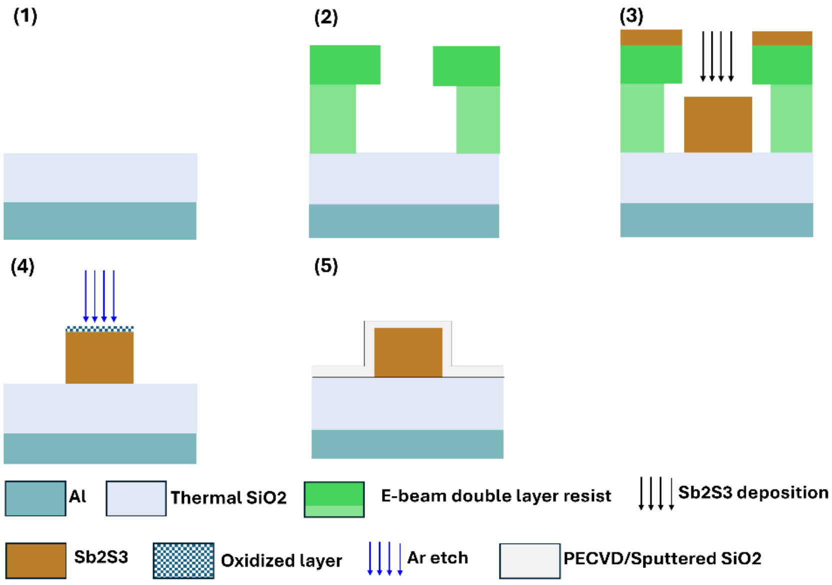


*Figure S8 Suggested fabrication process of the device*

The fabrication will be based on a lift-off process (Fig.S8). On a thoroughly cleaned, commercially available Si substrate, a 100 nm-thick Al layer will be coated (1). Next, a 60-nm-thick silica layer will be coated over the Al layer using electron beam evaporation. A bi-layer e-beam resist stack (MMA/PMMA) will then be spin-coated and exposed by electron-beam lithography (2). The use of a bilayer stack (MMA/PMMA) produces an undercut profile that facilitates a clean lift-off process and well-defined waveguide features. After development, the pattern will be treated with O2 and Ar plasma to improve the sample's surface adhesion and remove residual organics. Next,

approximately 320 nm of $Sb_2S_3$ is deposited by thermal evaporation at high vacuum (3) using pure $Sb_2S_3$ pellets (e.g., 99.99% based on Heeger Materials). The sample will be positioned directly above the evaporated material to ensure a nearly vertical flux for symmetrical waveguide sidewalls and minimal shadowing. Afterward, the sample will be placed in a solvent for lift-off. The sample with the formed $Sb_2S_3$ pattern is etched with Argon (Ar) plasma to the designed 300 nm height (4), removing organic contamination and oxidized surfaces. Without breaking the vacuum, a thin $SiO_2$ capping layer of thickness t is sputtered (5) to protect against oxidation and sulfide loss.

The lift-off technique offers several advantages for the $Sb_2S_3$-based fabrication, including reduced plasma-induced damage compared to direct etching and improved preservation of amorphous structure. However, the fabrication has its own limitations and drawbacks. Although we will suggest a thermal evaporator with a long working distance, previous experiments have shown that when samples are placed directly above the evaporated material, $Sb_2S_3$ strips tend to be angled, with rounded sidewalls, resulting in a trapezoidal profile. However, the trapezoidal profile can potentially be improved by increasing the evaporation distance or by using a single-layer resist and polishing. For instance, assuming slanted sidewalls of 80° with respect to the base, we simulate and present in Fig.9a,b the effect of the trapezoidal deformation of the strip. A reduction of ~5% (9%) could be expected, based on our simulation for an amorphous (crystalline) structure at a 45° incidence angle.

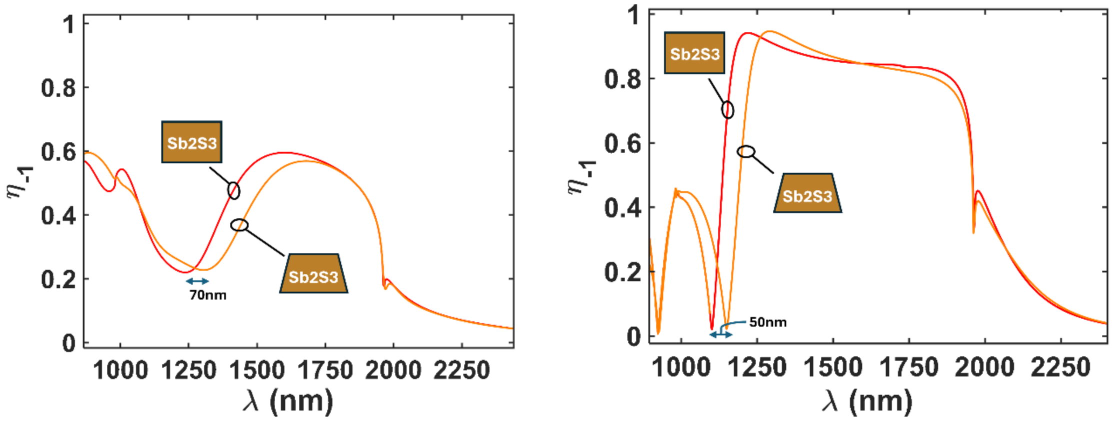


*Figure S9 Effect of trapezoid shape of the $Sb_2S_3$ strip on the performance of the device*

## Section E. Analysis of the deflection for the TM polarization

For sake of completeness, the analysis of device is also done under TM polarization of the incident wave. On one hand, Figure S10(a) shows the spectrum of the defection efficiency of the -1st order mode. Although one can notice a relatively high deflection efficiency, it presents ripples and a slow decaying cutoff at high wavelength. In the order, The -2nd order mode can be used for a narrow filter (e.g. around 1000 nm for $\theta = 60°$) as it has a narrow passband with a sharp cutoff, as shown in Fig.S10(b).

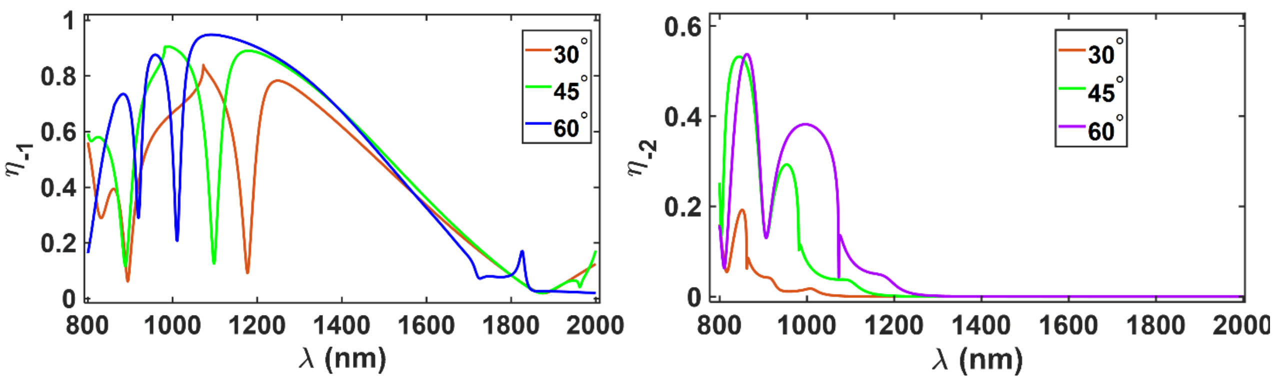


*Figure S10 Wavelength spectrum of the -1st order (a) and -2nd order (b) deflection coefficient. p=1150 nm, for $\theta_{inc}$ = 30°, 45° and 60°.*

## Section F. Electric and Magnetic field distribution at various incident angles

To elucidate the mode characteristics underlying the observed resonances, we examine the electric field (E-field) distribution under TE-polarized illumination. Figures S11–S12 compare the E-field around the nanorods in both crystalline and amorphous states at wavelengths of 1100, 1300, and 1600 nm, for incidence angles of 35° and 50°. The angle of 35° was chosen to prove the significant difference in deflection efficiency between the two phases (Fig. 2b in the main manuscript), while 50° corresponds to high-efficiency operation within the passband.

At 1300 and 1600 nm, the field distributions at both angles are similar, revealing the emergence of a tilted magnetic dipole when deflection efficiency is high. Moreover, the field patterns for amorphous and crystalline $Sb_2S_3$ are nearly identical, indicating that the increased loss (k) in the crystalline phase primarily accounts for the reduced efficiency. A notable difference appears at 1100 nm: in the amorphous phase, θ = 35° places the device near cutoff, with confinement to the $Sb_2S_3$ strip and an associated magnetic dipole, whereas θ = 50° moves the device away from cutoff, maximizing the field in the air above the structure.

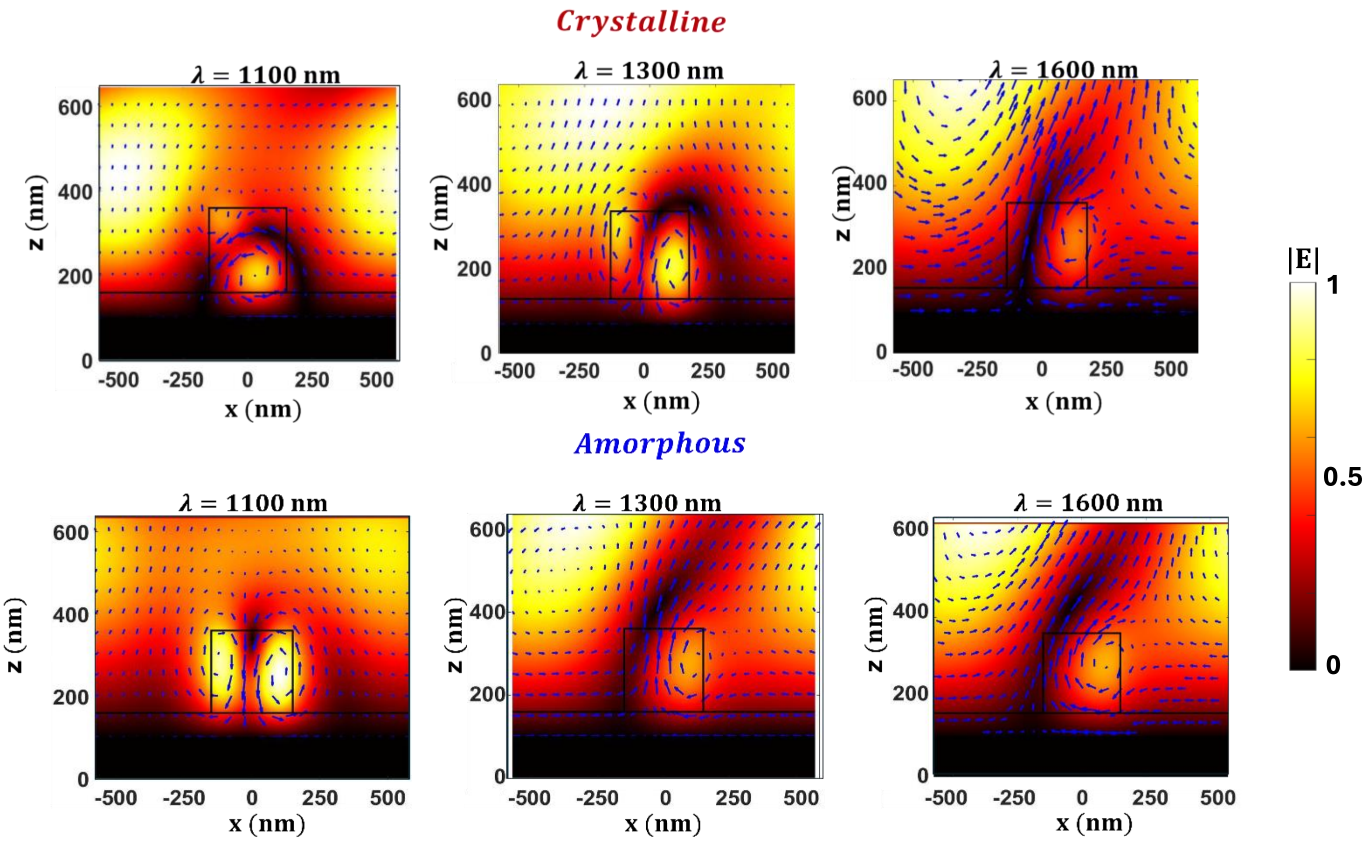


*Figure S11 contour plot of the electric field and the quiver plot of the magnetic field (overlap) for both crystalline and amorphous at θ= 35 °*

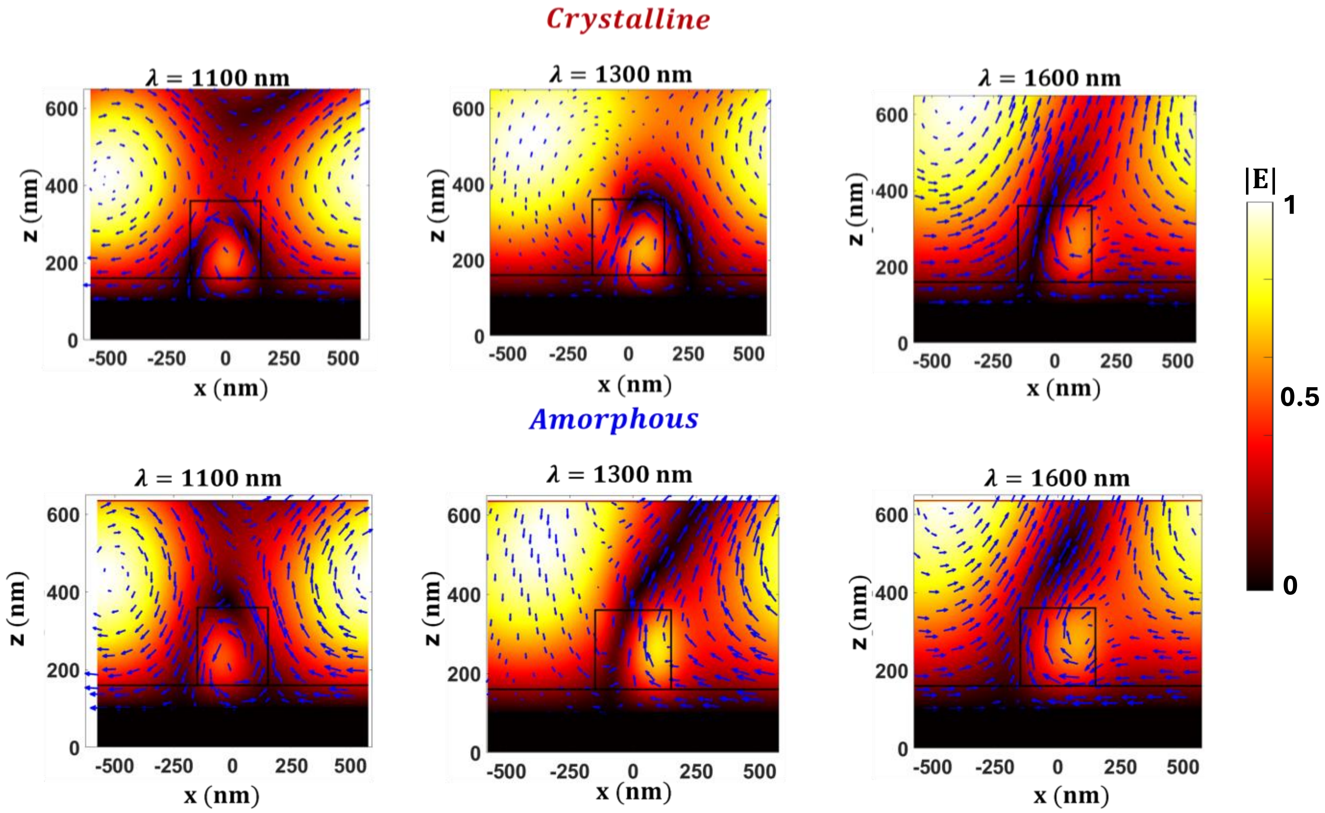


*Figure S12 contour plot of the electric field and the quiver plot of the magnetic field (overlap) for both crystalline and amorphous at $\theta = 50°$*

**Section G.**

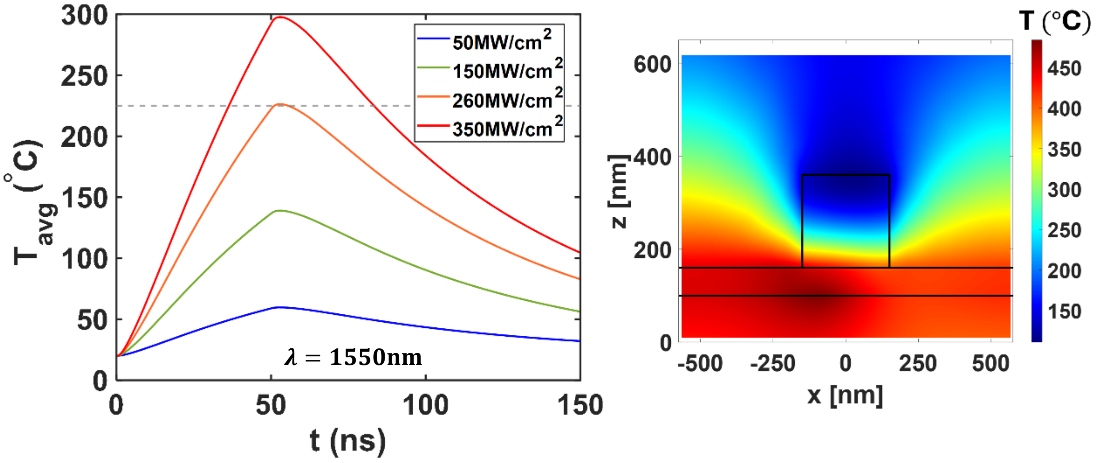


*Figure S13 (a) Change of the average temperature in the $Sb_2S_3$ strip with time, for different intensity of the incident wave. The dash line represents the temperature for phase changing from amorphous to amorphous crystalline. (right) Temperature distribution in a unit cell cross section of the device for a pulse laser intensity of 260 $MW/cm^2$ at 50ns; $\lambda = 1550nm$.*

The dynamic configurability of our device is enabled by antimony trisulfide ($Sb_2S_3$), a phase-change material that can be reversibly switched between amorphous and crystalline states via thermal heating or continuous-wave optical excitation. The amorphous-to-crystalline transition occurs at ~225 °C [1], allowing the device to operate in two distinct regimes: a **normal mode** based on the amorphous phase, and a low efficiency/**attenuation mode** based on the crystalline phase. At elevated optical intensities, the temperature of the $Sb_2S_3$ strip rises over time, driving a self-initiated phase transition once the critical temperature is reached. Figure 1a illustrates the temporal evolution of the average temperature under increasing optical intensity, obtained from coupled electromagnetic and thermal simulations in CST. Under a 50 ns pulse, at 1550 nm wavelength, emulating a pulsed laser, an intensity of ~260 MW/cm$^2$ is required to raise the strip to 225 °C. The relatively high intensity threshold is since Sb2S3 has very low absorption (see n,k data below(Fig.S5)) in the region of interest. Considering that the change of temperature depends on fluece, a longer exposition (>50ns) will reduce the threshold. The corresponding spatial temperature distribution across the device cross-section is shown in Fig. S13b.

**<u>References</u>**:

1. K. Aryana, H. J. Kim, M. R. Islam, N. Hong, C.-C. Popescu, S. Makarem, T. Gu, J. Hu, and P. E. Hopkins, “Optical and thermal properties of Ge2Sb2Te5, Sb2Se3, and Sb2S3 for reconfigurable photonic devices [Invited],” *Opt. Mater. Express* **13**, 3277–3286 (2023).

2. J. Feldmann, N. Youngblood, C. D. Wright, H. Bhaskaran, and W. H. P. Pernice, “Ultra-low-energy programmable non-volatile silicon photonics based on phase-change materials with graphene heaters,” *Nat. Commun.* **12**, 246 (2021).

3. Z. Cheng, M. Caldarola, C. Li, H. Hu, T. He, S. Raza, *et al.*, “Sb2S3 as a low-loss phase-change material for mid-IR photonics,” *Opt. Mater. Express* **13**, 4707–4718 (2023).

4. M. Kong, H. Lyu, Y. Zhang, J. Zheng, C. Li, H. Hu, *et al.*, “Capping layer effects on Sb2S3-based reconfigurable photonic devices,” *ACS Photonics* **10**, 3203–3214 (2023).

5.C. Li, T. He, H. Hu, Z. Cheng, M. Caldarola, S. Raza, *et al.*, “Low-loss Sb2S3 optical phase shifter enabled by optimizing sputtering conditions,” *Opt. Mater. Express* **14**, 1472–1482 (2024).

6. M. Delaney, I. Zeimpekis, D. Lawson, D. W. Hewak, and O. L. Muskens, "A new family of ultralow loss reversible phase-change materials for photonic integrated circuits: Sb2S3 and Sb2Se3," Adv. Funct. Mater. **30**, 2002447 (2020)
